# Supplementary material for: AlignGen: Boosting Personalized Image Generation with Cross-Modality Prior Alignment
Source: arXiv:2505.21911 source file (2025-05-28)
Supplement: Supplementary file 1 [file supp.tex]

\clearpage
\setcounter{page}{1}
\appendix

\section{Implementation Details}
% \subsection{Framework}

\subsection{Training Settings} 
\noindent\textbf{Setting of Image Size.}The target and reference image sizes are both set to $512\times512$. 

\noindent\textbf{Setting of LoRA.} The reference image shares the same VAE and DiT layers with the target image. LoRA \cite{hu2022lora} is applied exclusively to the reference image, affecting the image embedder, the query/key/value linear layers, and the feed-forward layer. LoRA parameters are initialized using a Gaussian distribution. To maintain the model's original capabilities, the LoRA scale is set to 0 when processing noisy image tokens.

\subsection{Evaluation Settings}
\noindent\textbf{Training Settings.} For test-time optimization methods, such as Textual Inversion \cite{gal2023an}, DreamBooth \cite{ruiz2023dreambooth}, and DreamBooth LoRA \cite{ruiz2023dreambooth}, we need to train them for each image in the benchmark. As detailed in Table \ref{tab:training_setting_tto}, we adhere to the training settings specified in DreamBench++ \cite{peng2024dreambench}.

\begin{table}[h]
\centering
\caption{Training settings of test-time optimization methods. BS: batch size, LR: learning rate, Steps: training steps.}
\begin{tabular}{c|ccc}
\toprule 
 Method  & BS & LR & Steps  \\ \midrule
 Textual Inversion \cite{gal2023an} & 1          & 5e-4          & 3000 \\
 DreamBooth \cite{ruiz2023dreambooth} & 1          & 2.5e-6           & 250 \\
 DreamBooth LoRA \cite{ruiz2023dreambooth} & 1          & 5e-5           & 500 \\

\bottomrule
\end{tabular}
\label{tab:training_setting_tto}
\end{table}

\noindent\textbf{Inference Settings.}
The seed, guidance scale, and number of inference steps used in our experiments are summarized in Table \ref{tab:inference_table}. For OmniControl \cite{tan2024ominicontrol} and Diffusion Self-Distillation \cite{cai2024diffusion}, we adopt the official implementations. All other methods follow the settings provided in DreamBench++. Note that OmniControl offers multiple checkpoint versions; we use the \href{https://huggingface.co/Yuanshi/OminiControl/tree/main/omini}{omini/subject\_512 model}, which has been fine-tuned on a larger dataset and demonstrates superior performance compared to the version reported in the original paper. For OmniControl , only 8 inference steps are conducted, as its base text-to-image model is FLUX.1-Schnell \cite{flux2024}.

\begin{table}[h]
\centering
\caption{Inference settings of different methods. GS: guidance scale, Steps: inference steps.}
\begin{tabular}{c|ccc}
\toprule
 Method  & Seed & GS & Steps  \\ \midrule
 Textual Inversion \cite{gal2023an} & 42          & 7.5          & 100 \\
 DreamBooth \cite{ruiz2023dreambooth} & 42          & 7.5          & 100 \\
 DreamBooth LoRA \cite{ruiz2023dreambooth} & 42          & 7.5          & 100 \\
 IP-Adapter ViT-G \cite{ye2023ip} & 42          & 7.5          & 100 \\
 IP-Adapter-Plus ViT-H \cite{ye2023ip} & 42          & 7.5          & 100 \\
 BLIP-Diffusion \cite{li2023blip} & 42          & 7.5          & 100 \\
 Emu2 \cite{sun2024generative} & 42          & 3          & 50 \\
 OminiControl \cite{tan2024ominicontrol} & 42          & 3.5          & 8 \\
 Diffusion Self-Distillation \cite{cai2024diffusion}   & 42          & 3.5          & 28 \\
 Ours & 42          & 3.5          & 28 \\
\bottomrule
\end{tabular}
\label{tab:inference_table}
\end{table}

\section{Image Description Rewrite}
To improve robustness to variations in concept terminology, we introduce a training strategy that randomly replaces a target concept name (e.g., acoustic guitar) with either its parent class or a broader category (e.g., musical instrument). However, the Subject200K dataset \cite{tan2024ominicontrol} provides limited lexical diversity for target concept names. To address this limitation, we employ DeepSeekV3 \cite{deepseekai2024deepseekv3technicalreport} to rewrite image descriptions. Specifically, we prompt the model to replace the target concept with a placeholder token $\langle$concept$\rangle$ in the image description and to output both the parent class and a broader category. The prompt template used for this rewriting process is shown in Figure~\ref{fig:prompt_rewirte}.

\begin{figure*}
    \centering
    \includegraphics[width=0.9\textwidth]{samples/supp/prompt_rewrite.pdf}
    \caption{Illustration of the specific prompt employed by DeepSeekV3 to alter image descriptions within the Subject200K dataset.}
    \Description{Illustration of the specific prompt employed by DeepSeekV3 to alter image descriptions within the Subject200K dataset.}
    \label{fig:prompt_rewirte}
\end{figure*}

\section{More Visualizations}
Due to space constraints in the main paper, we provide more qualitative results in Figure \ref{fig:visualization_supp_1}, Figure \ref{fig:visualization_supp_2}, including objects, animals, and humans.

\begin{figure*}
    \centering
    \includegraphics[width=0.9\textwidth]{samples/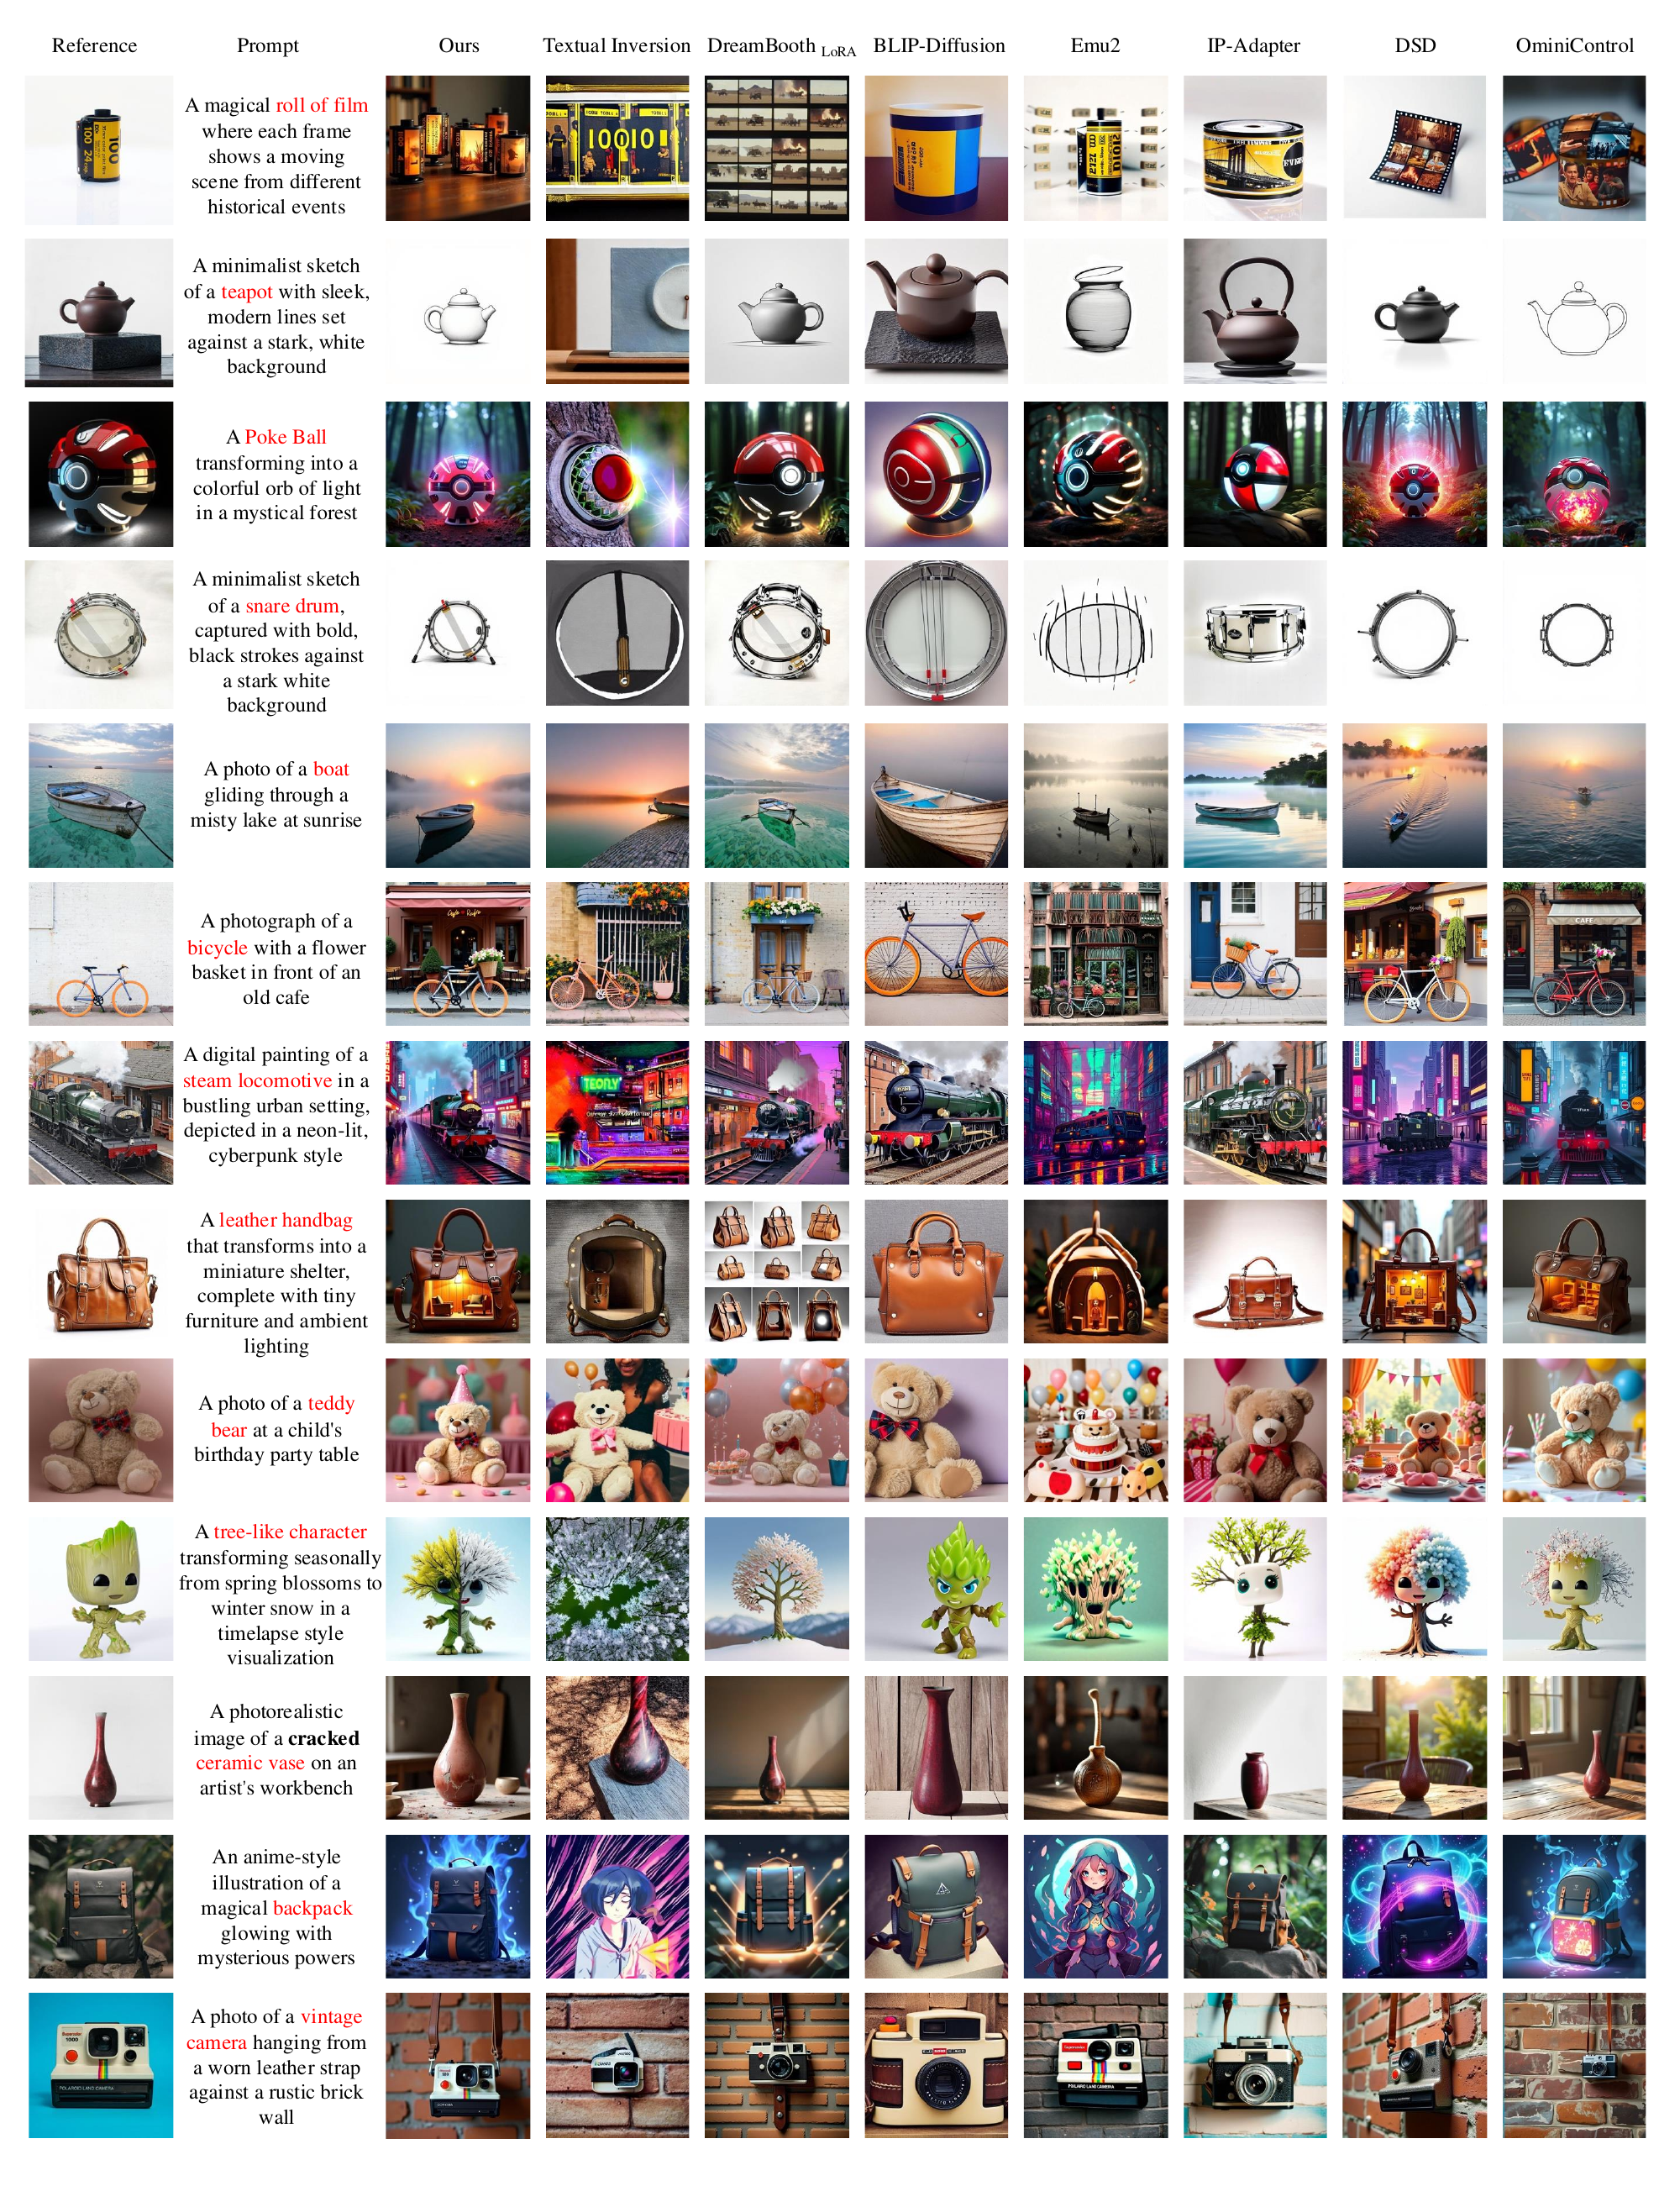}
    \caption{Qualitative comparison of the results on the Dreambench++ benchmark.}
    \Description{Qualitative comparison of the results on the Dreambench++ benchmark.}
    \label{fig:visualization_supp_1}
\end{figure*}

\begin{figure*}
    \centering
    \includegraphics[width=0.9\textwidth]{samples/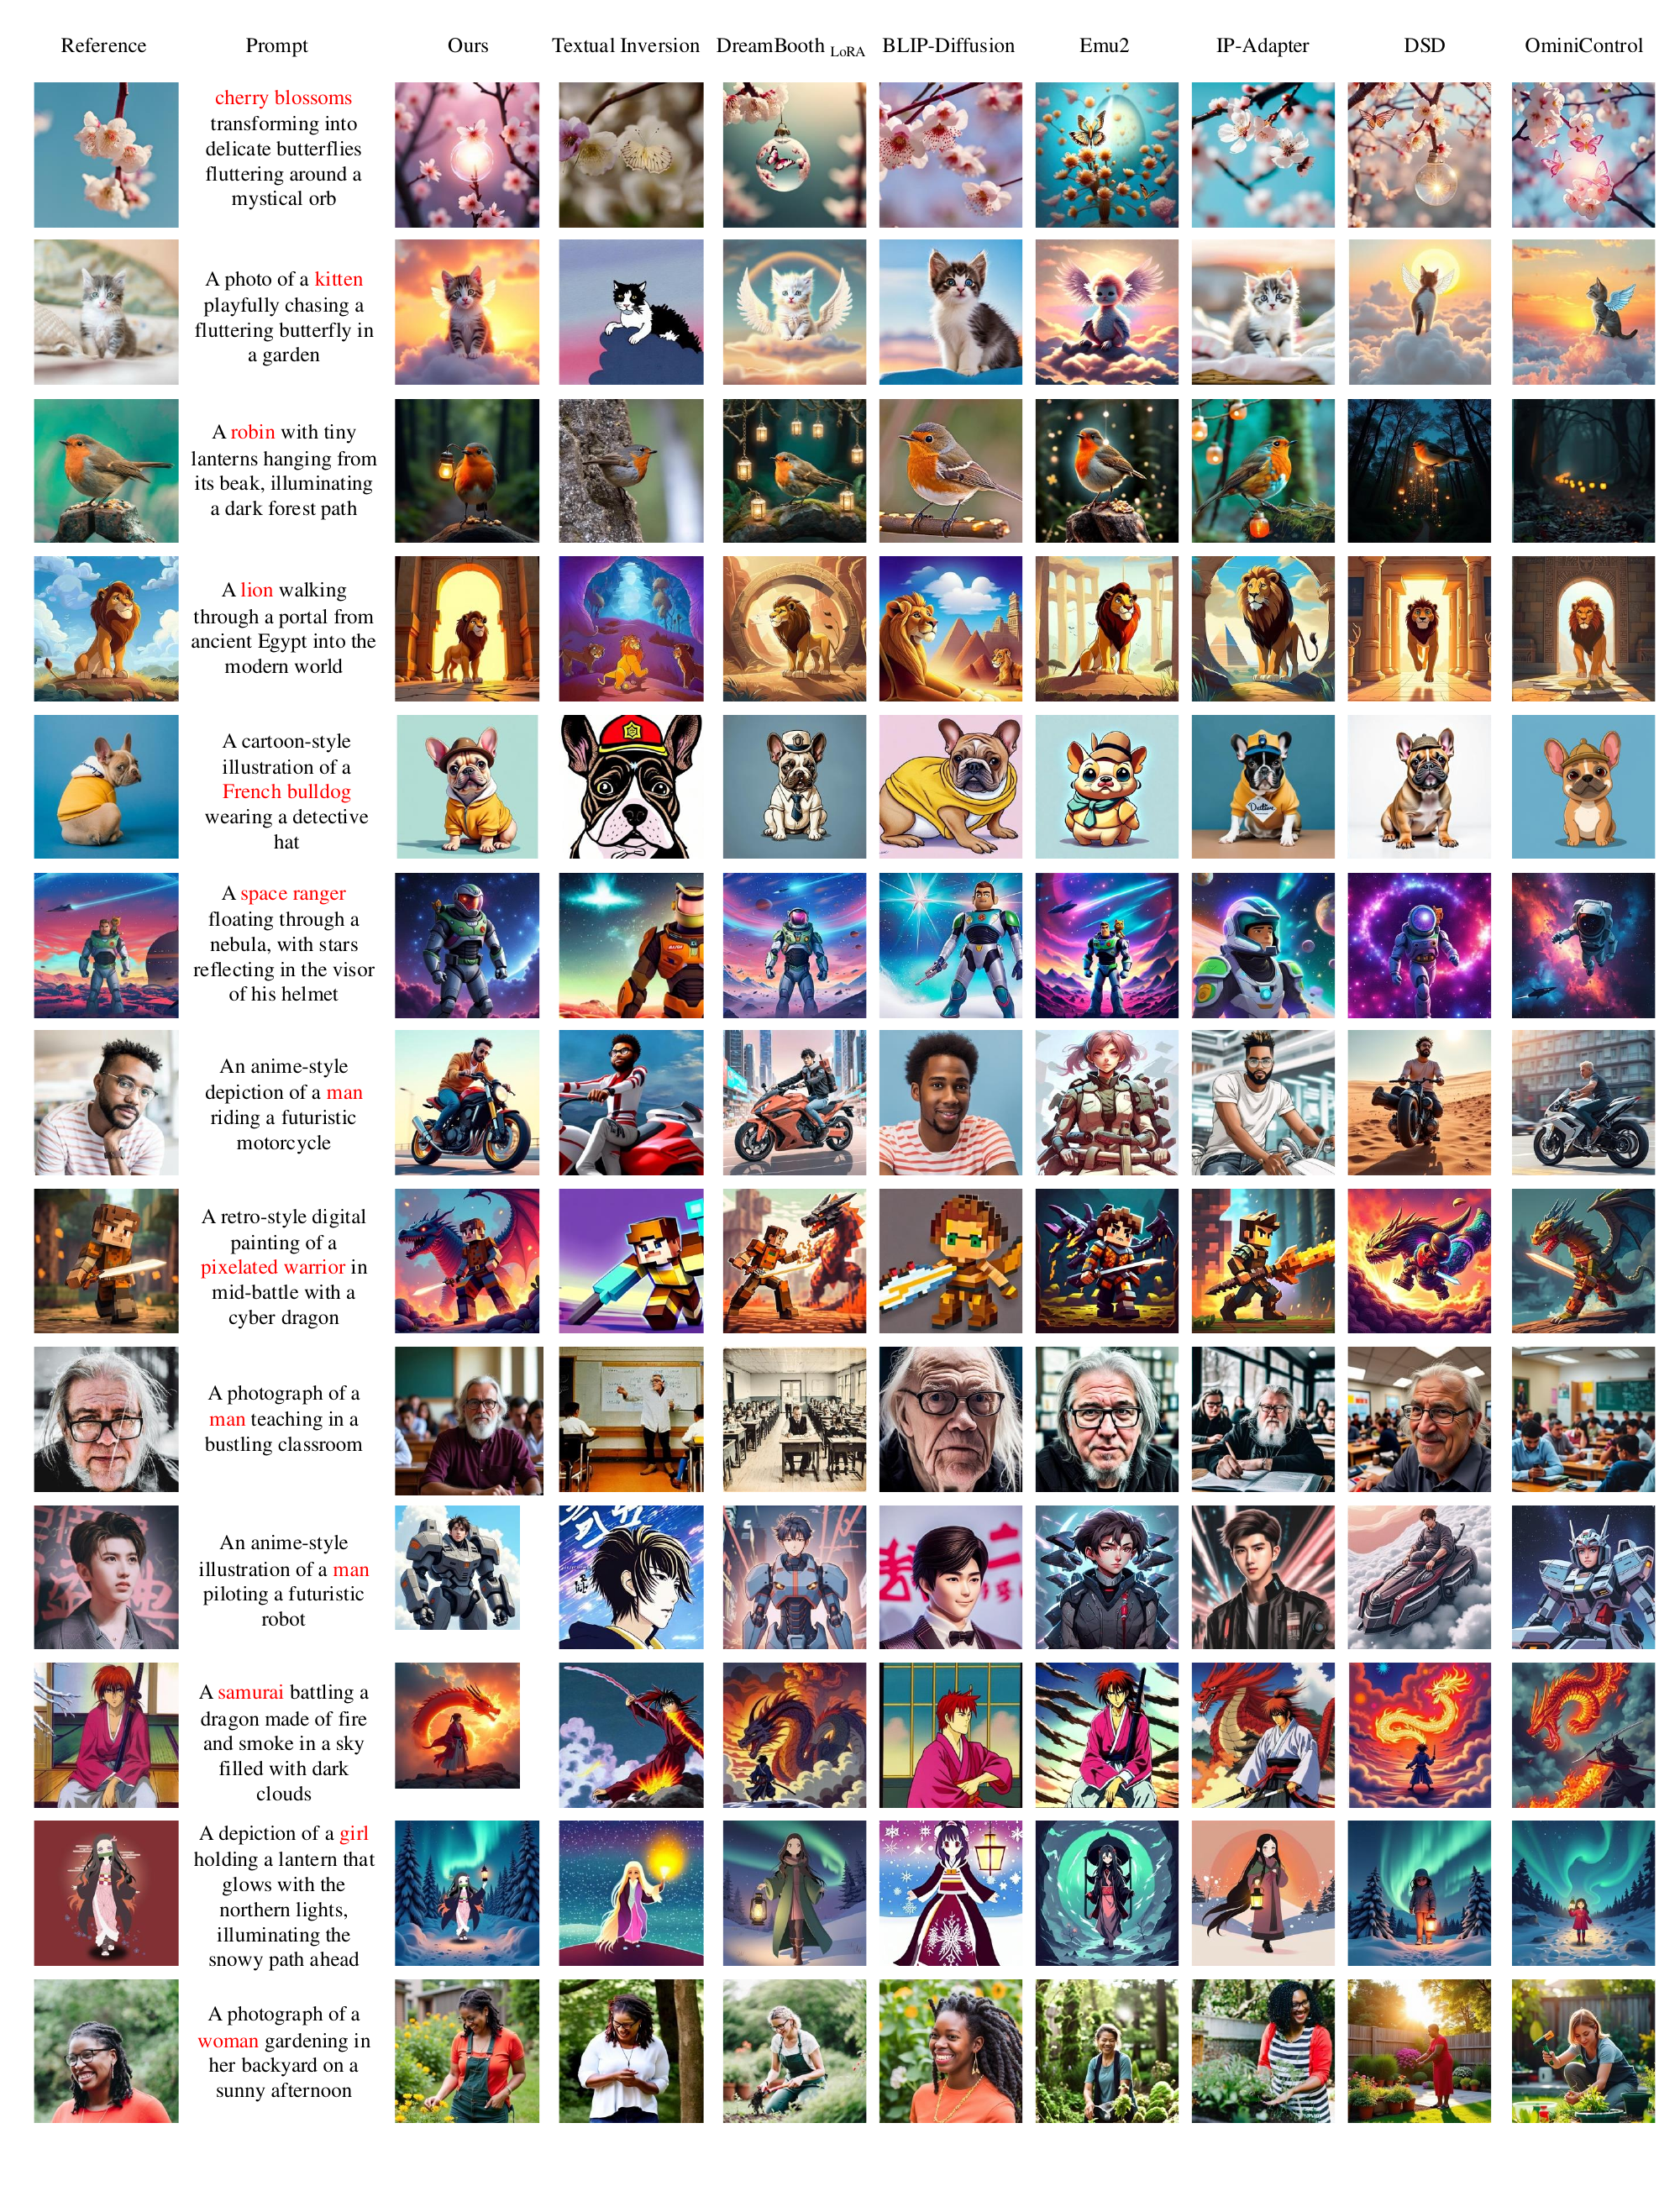}
    \caption{Qualitative comparison of the results on the Dreambench++ benchmark.}
    \Description{Qualitative comparison of the results on the Dreambench++ benchmark.}
    \label{fig:visualization_supp_2}
\end{figure*}
