# Supplementary material for: AlignGen: Boosting Personalized Image Generation with Cross-Modality Prior Alignment
Source: arXiv:2505.21911 source file (2025-05-28)
Supplement: Supplementary file 2 [file prompt_rewrite.tex]

\begin{figure*}
    \centering
    \includegraphics[width=0.9\textwidth]{samples/supp/prompt_rewrite.pdf}
    \caption{Illustration of the specific prompt employed by DeepSeekV3 to alter image descriptions within the Subject200K dataset.}
    \Description{Illustration of the specific prompt employed by DeepSeekV3 to alter image descriptions within the Subject200K dataset.}
    \label{fig:prompt_rewirte}
\end{figure*}
